# Supplementary material for: Policy Teaching via Environment Poisoning: Training-time Adversarial Attacks against Reinforcement Learning
Source: arXiv:2003.12909 source file (2020-08-19)
Supplement: Supplementary file 1 [file 9.5_appendix_misc.tex]

% !TEX root =  main.tex
%%%%%%%%%%%%%%%%%%%%%%%%%%%%%%%%%%%%%
%%%%%%%%%%%%%%%%%%%%%%%%%%%%%%%%%%%%%
% !TEX root =  main.tex
%%%%%%%%%%%%%%%%%%%%%%%%%%%%%%%%%%%%%
%%%%%%%%%%%%%%%%%%%%%%%%%%%%%%%%%%%%%
\section{Misc}
%: Known MDP
\subsection{GORAN --- Proof of General Ideas in Section \ref{sec.on.known.ideas}}

\paragraph{Proof of Proposition \ref{prop.on.known.nontarget}}
Assume the learner follows an algorithm $\mathfrak{A}$ which chooses the action from a distribution based on the previous observations. Theorem 5.5.1 in \cite{Puterman1994} shows that a history-independent algorithm $\Pi$ exists that chooses the action $a_t$ form the distribution $q_{t, s_t}$ where the distributions $q_{t,s}$ are fixed and we have
\begin{gather}
\label{equal_dist}
    \forall s,a,t: \Pru{\mathfrak{A}}{s_t =s, a_t = a} =  \Pru{\Pi}{s_t =s, a_t = a},\\
    \label{equal_decision}
    q_{t,s}(a) = \Pru{\mathfrak{A}}{a_t = a | s_t = s}.
\end{gather}

Equation (\ref{equal_dist}) means $\Pi$ has the same expected regret and non-target actions as $\mathfrak{A}$. Thus it suffices to prove the theorem for $\Pi$.

First, we extend the definitions of $P$, $R$, and $Q$ defined in Appendix \ref{appendix_background} as
\begin{gather*}
    Q(s, d) = \expctu{a\sim d}{Q(s, a)}\\
    R(s, d) = \expctu{a\sim d}{R(s, a)}\\
    P(s, d, s') = \expctu{a\sim d}{P(s, a, s')}
\end{gather*}{}
for distribution $d$ on the actions.

Now let $M = (\cS, \cA, R, P)$ be the environment. Denote the $Q$ values, $V$ values, and average reward of $\pi$ on $M$ by $Q^{\pi}$, $V^{\pi}$, and $\rho^*$ as $\pi$ is $\epsilon$-robust optimal on $M$. By Corollary \ref{gain_diff_neighbor} we have
\begin{align*}
    V^{\pi}(s) - Q^{\pi}(s, a)&= 
    \frac{1}{\mu^{\pi\bracket{s,a}}_0(s)}\big(
    \rho^* - \rho^{\pi\bracket{s,a}}
    \big)\\
    &\ge \frac{\epsilon}{\overline{\mu}}
\end{align*}{}
Defining $\eta = \epsilon/\overline{\mu}$, we can write
\begin{align*}
    Q^{\pi}(s, q_{t,s}) &= \sum_{a\ne\pi(s)} q_{t,s}(a)Q^{\pi}(s,a) + q_{t,s}(\pi(s))V^{\pi}(s)\\
    &\le \sum_{a\ne\pi(s)} q_{t,s}(a)\big(V^{\pi}(s) - \eta\big) + q_{t,s}(\pi(s))V^{\pi}(s)\\
    &= V^{\pi}(s) - \eta\bigg(1 - q_{t,s}(\pi(s))\bigg)\\
    &= V^{\pi}(s) - \eta e_{t,s},
\end{align*}{}
defining $e_{t,s} = 1 - q_{t,s}(\pi(s))$. Using the definition of $Q^{\pi}$ we have
\begin{align*}
    R(s, q_{t,s}) + \sum_{s'}P(s, q_{t,s}, s')V^{\pi}(s') - V^{\pi}(s) + \eta e_{t,s} \le \rho^*.
\end{align*}{}
Note that since the target policy is the optimal policy we denoted its average reward as $\rho^*$. This can be written in vector notation as
\begin{align*}
    R_{q_t} + (P_{q_t} - I)V^{\pi} + \eta e_t \le \rho^*\mathbf 1.
\end{align*}
Now let $d_t(s) = \Pru{\Pi}{s_t = s}$, and $d_t$ be the row vector of that. Thus, $d_{t+1} = d_{t} P_{q_t}$.
Multiplying the last inequality by $d_t$ from left gives
\begin{align*}
    &d_{t}R_{q_t} + (d_{t+1} - d_t)V^{\pi} + \eta  d_t e_t \le \rho^*\\
    \Rightarrow & \eta  d_t e_t \le \rho^* - \expct{r_t} + (d_t - d_{t+1})V^{\pi}.
\end{align*}
Summing the inequality for $t = 1$ to $T$:
\begin{align*}
    \eta\sum_{t=1}^T d_t e_t &\le T\rho^* - \expct{\sum_{t=1}^T r_t} + (d_0 - d_{T+1})V^{\pi}\\
    &\le m(T) + 2\norm{V^{\pi}}_\infty
\end{align*}{}

\goran{
Assuming we want to adopt the following notion of cost:
\begin{align*}
    \varphi(T) = \sum_{t} \frac{1}{|\cS|} \sum_s \mathds 1_{\pi_t \ne \pi_T(s)} 
\end{align*}{}
would something along these lines be useful? 
 ------------START --------
}

\begin{align*}
  &\expct{\sum_{t} \frac{1}{|\cS|} \sum_s \mathds 1_{\pi_t \ne \pi_T(s)}} = O(\tau) +  \frac{1}{|\cS|} \sum_{t > \tau}  \sum_s \frac{d_t(s)}{d_t(s)} e_{t,s} \le O(\tau) +  \frac{1}{|\cS| \mu_*} \sum_{t > \tau}  \sum_s d_t(s) e_{t,s}
  \\&\le O(\tau) +  \frac{1}{|\cS| \cdot (\mu_* - \epsilon)} \sum_{t}  \sum_s d_t(s) e_{t,s} \le O(\tau) + \frac{1}{|S|\cdot (\mu_* - \epsilon)}(m(T) + 2 \cdot \norm{V^\pi}_{\infty})
\end{align*}{}
where $\tau$ is such that $d_t(s) \ge  \mu_* - \epsilon$ for $t > \tau$, and $\epsilon << \mu_*$. When we are changin rewards only, it seems that $\mu_*$ and $\tau$ can be found by combining diameter $D_0$ of MDP $M_0$ and mixing time. Diameter should provide $\mu_*$, e.g., $\mu_* = \frac{1}{D_0}$. A useful bound on $t_{mix}$ is (please double-check!):
\begin{align*}
    t_{mix}(\epsilon') \le t_{rel} \cdot \log \frac{1}{2 \cdot \mu_*^{1/2} \cdot \epsilon'} 
\end{align*}
$\epsilon' = \epsilon/|\cS|$ and $t_{rel} = \frac{1}{1-\lambda^*}$, where $\lambda^*$ is the sub-radius.  According to Putterman $\lambda^* \le 1 - \alpha$, so we have:
\begin{align*}
    t_{mix}(\epsilon') \le \frac{1}{\alpha} \cdot \log \frac{D_0^{1/2} \cdot |S|}{2 \cdot \epsilon}
\end{align*}
And so $\tau$ could be equal to $\tau = t_{mix}$, while $\mu_* = \frac{1}{D_0}$. Unfortunately, it's not clear if this idea would even work when we perform attacks on dynamics (e.g., how to ensure a bound on $D_0$?). 

\goran{
-------------END ------------
}

Now note that
\begin{align*}
    \sum_{t=1}^T d_t e_t &= \sum_{t=1}^T \sum_s d_t(s) e_{t,s}\\
    &= \sum_{t=1}^T \sum_s \Pr{s_t = s} \bigg(1 - q_{t,s}(\pi(s))\bigg)\\
    &= \sum_{t=1}^T \sum_s \Pr{s_t = s} \Pr{a_t \ne \pi(s_t) | s_t = s}\\
    &= \sum_{t=1}^T \Pr{a_t \ne \pi(s_t)}\\
    &= \expct{\varphi(T)}.
\end{align*}{}
Therefore, we have 
\begin{align*}
    \expct{\varphi(T)} &\le \frac{m(T) + 2\norm{V^{\pi}}_\infty}{\eta}\\
    &= \frac{\overline{\mu}}{\epsilon}\Big(m(T) + 2\norm{V^{\pi_T}_0}_\infty\Big).
\end{align*}{}

\goran{Maybe add a sentence to clarify where $V^{\pi_T}_0$ comes from (is $V^{\pi_T} = V^{\pi_T}_0$ throughout the proof?)}\amin{The zero was a typo. It is a general claim apart from proofs of the theorems. I have mentioned that these are Q,V values in the environment }

\amin{Better reasoning for not altering target actions and a better goal.}
Let $N_s(t)$ denote the number of times state $s$ is visited in the first $T$ steps, and $M_{s, a}(n)$ be number of times actions $a$ is taken from state $s$ in the first $n$ visits to state $s$.

\begin{lemma}
If we have $\expct{\missm(T)} = \smallObound(T)$ and $\expct{N_s(T)} = \Omegabound(T)$ for some state $s$, then $\expct{M_{s, \targetpi(s)}(n)} = \Thetabound(n)$.
\end{lemma}{}

\begin{proof}
We have \begin{align*}
\expct{M_{s, \targetpi(s)}(N_s(T))} &= N_s(T) - 
\sum_{a \ne \targetpi(s)}\expct{M_{s, a}(N_s(T))} \\
&\le \sum_{s \in S} \sum_{a \ne \targetpi(s)} \expct{M_{s,a}(N_s(T))}\\
&= \expct{\missm(T)}\\
&= \smallObound(T)
\end{align*}

\end{proof}{}

\begin{lemma}
If the attacker guarantees sublinear expected number of missmatches as $\expct{\missm(T)} = \smallObound(T)$, with sublinear expected cost as $\expct{\cost(T)} = \smallObound(T)$, then all the states are visited linear number of times in expectation, i.e., $\expct{N_s(T)} = \Omegabound(T)$ for every state $s$.
\end{lemma}

\begin{proof}
Consider the partition of $S = X \cup Y$ such that 
$X = \{s | \expct{N_s(T)} = \Omegabound(T)\}$ and $Y = \{s | \expct{N_s(T)} = \smallObound(T)\}$. For every $s \in A$ 
\end{proof}{}

\begin{proposition}
If the attacker achieves sublinear expected number of missmatches as $\expct{\missm(T)} = \smallObound(T)$, with sublinear expected cost as $\expct{\cost(T)} = \smallObound(T)$, then for any state $s$, the target action $\targetpi(s)$ is almost always played from $s$. More specifically, we have $M_{s, \targetpi(s)}(n) = \Thetabound(n)$ .
\end{proposition}{}

\begin{proposition}
Assume the attacker achieves sublinear expected number of missmatches as $\expct{\missm(T)} = \smallObound(T)$ by simulating an ergodic MDP $\hat{M} = (S, A, \hat{R}, \hat{P})$. If for some state $s$ we have $\hat{P}(s, \targetpi(a), .) \ne \overline{P}(s, \targetpi(s), .)$ or $\hat{R}(s, \targetpi(s)) \ne \overline{R}(s, \targetpi(s))$, then $\expct{\cost(T)} = \Omegabound(T)$
\end{proposition}{}
